# Supplementary material for: Advances in Automatically Rating the Trustworthiness of Text Processing Services
Source: arXiv:2302.09079 source file (2023-02-04)
Supplement: Supplementary file 1 [file appendix_rough.tex]

\section{Random Stuff}

\cite{zeiler2013visualizing} visualises the internal representation learned by CNNs using deconvolutional networks. Other approaches have attempted to synthesise an input that highly stimulates a neuron, such as \cite{simonyan2014deep, nguyen2016synthesizing, yosinski2015understanding}. There are numerous examples of combining the layer activation maps with the gradient information to investigate saliency computation utilising various layers of deep models. GradCAM \cite{Selvaraju_2019}, a generalised variant of CAM \cite{zhou2015learning}. All of the approaches mentioned above require access to the underlying model’s internals to acquire feature activation values, gradients, or weights.

Several studies have shown that certain backpropagation-based approaches produce the same saliency map regardless of the output neuron or network characteristics evaluated \cite{adebayo2020sanity, Mahendran_2016}. As a result, these methods may be able to characterise average network features but not individual outputs or intermediate activations in some cases.

Another strategy involves changing the inputs to a model and seeing the changes in the outputs as a result. Occlusion \cite{zeiler2013visualizing} occlude an image using regular occlusion patterns and weight the changes in the output by occlusion pattern. Meaningful perturbations \cite{Fong_2017} optimise a spatial perturbation mask that has the most impact on a model's output. With a second neural network, real-time saliency \cite{dabkowski2017real} learns to predict such a perturbation mask. Other studies have used \cite{singh2017hideandseek} perturbations at the input. LIME \cite{ribeiro2016why} approximates the deep model with a linear classifier, trains it at the input point with samples with occluded superpixels, and uses the weights acquired as a metric of superpixel significance. RISE \cite{petsiuk2018rise} builds a set of random masks, applies the classifier to masked copies of the input, weights the predicted class probabilities, and computes the saliency map as a weighted sum of the masks.

However, as in the case of image classification, the methods discussed above can only justify scalar numbers, or class probabilities. In addition to class probabilities, an object detector would additionally predict an object's bounding box location, which needs explanations. It also creates numerous detection suggestions per image, which may differ significantly for perturbed image copies. Because of these inconsistencies, existing classification saliency algorithms cannot be used directly. We solve these concerns in our research, allowing object detectors to generate saliency maps. We use the RISE masking approaches in our work with modifications to feasibly compute the explanation for object detection.
